# Supplementary material for: Mobilizing Personalized Federated Learning in Infrastructure-Less and Heterogeneous Environments via Random Walk Stochastic ADMM
Source: arXiv:2304.12534 source file (2023-09-26)
Supplement: Supplementary file 1 [file references_appendix.tex]

%%%%%%%%%%%%%%%%%%%%%%%%%%%%%%%%%% Author's 
@book{rockafellar2009variational,
  title={Variational analysis},
  author={Rockafellar, R Tyrrell and Wets, Roger J-B},
  volume={317},
  year={2009},
  publisher={Springer Science \& Business Media}
}

@article{chung1952application,
  title={On the application of the Borel-Cantelli lemma},
  author={Chung, Kai Lai and Erdos, Paul},
  journal={Transactions of the American Mathematical Society},
  volume={72},
  number={1},
  pages={179--186},
  year={1952},
  publisher={JSTOR}
}

@article{hu2023stochastic,
  title={Stochastic linearized generalized alternating direction method of multipliers: Expected convergence rates and large deviation properties},
  author={Hu, Jia and Guo, Tiande and Han, Congying},
  journal={Mathematical Structures in Computer Science},
  pages={1--18},
  year={2023},
  publisher={Cambridge University Press}
}
